# Supplementary material for: Noisy-Input Entropy Search for Efficient Robust Bayesian Optimization
Source: arXiv:2002.02820 source file (2020-02-07)
Supplement: Supplementary file 1 [file supplementary.tex]

\documentclass[twoside]{article}

\usepackage{aistats2020}

\usepackage[square, numbers]{natbib}

\usepackage[utf8]{inputenc} %
\usepackage[T1]{fontenc}    %
\usepackage{url}            %
\usepackage{booktabs}       %
\usepackage{amsfonts}       %
\usepackage{nicefrac}       %
\usepackage{microtype}      %
\usepackage{amsmath}
\usepackage{algorithm}
\usepackage{algpseudocode}
\usepackage{eqparbox}

\usepackage{graphicx}
\usepackage{subcaption}
\usepackage{bm}
\usepackage{bbm}
\usepackage{color}
\usepackage[shortlabels]{enumitem}
\usepackage{tikz}
\usepackage{pgfplots}
\usetikzlibrary{pgfplots.groupplots}
\usetikzlibrary{shapes}
\usepackage{tabularx}
\usepackage{todonotes}
\usepackage{multirow}
\usepackage{glossaries}
\usepackage{todonotes}
\usepackage{wrapfig}
\usepackage{lipsum}

\glsdisablehyper

\definecolor{tableauC0}{rgb}{0.122, 0.467, 0.706}
\definecolor{tableauC1}{rgb}{1.000, 0.500, 0.055}
\definecolor{tableauC2}{rgb}{0.172, 0.627, 0.172}
\definecolor{tableauC3}{rgb}{0.839, 0.153, 0.157}
\definecolor{tableauC4}{rgb}{0.578, 0.402, 0.738}
\definecolor{tableauC5}{rgb}{0.547, 0.336, 0.293}
\definecolor{tableauC6}{rgb}{0.887, 0.465, 0.759}
\definecolor{tableauC7}{rgb}{0.500, 0.500, 0.500}
\definecolor{tableauC8}{rgb}{0.734, 0.738, 0.133}

\tikzset{cross/.style={cross out, draw=black, minimum size=2*(#1-\pgflinewidth), inner sep=0pt, outer sep=0pt}, cross/.default={1pt}}

\newcolumntype{Y}{>{\centering\arraybackslash}X}

\newacronym{acr:bo}{BO}{Bayesian optimization}
\newacronym{acr:ei}{EI}{expected improvement}
\newacronym{acr:ep}{EP}{expectation propagation}
\newacronym{acr:es}{ES}{entropy search}
\newacronym{acr:gp}{GP}{Gaussian process}
\newacronym{acr:ir}{IR}{inference regret}
\newacronym{acr:kde}{KDE}{kernel density estimate}
\newacronym{acr:mes}{MES}{max-value entropy search}
\newacronym{acr:nes}{NES}{Noisy-Input Entropy Search}
\newacronym{acr:pes}{PES}{predictive entropy search}
\newacronym{acr:pi}{PI}{probability of improvement}
\newacronym{acr:rs}{RS}{rejection sampling}
\newacronym{acr:se}{SE}{squared exponential}
\newacronym{acr:ssgp}{SSGP}{sparse spectrum Gaussian process}
\newacronym{acr:ucb}{UCB}{upper confidence bound}

\begin{document}

 \twocolumn[
 
 \aistatstitle{Supplementary Material: \\Noisy-Input Entropy Search\\for Efficient Robust Bayesian Optimization}
 
 \aistatsauthor{Anonymous Author(s)}
 \aistatsaddress{Affiliation} ]
 
 \appendix
 \newcommand{\axisheight}{1.0\linewidth}
 \newcommand{\axiswidth}{1.12\linewidth}
 \newcommand{\subfigurewidth}{.32\linewidth}
 \newcommand{\captionvspace}{-2mm}
 \newcommand{\axisheightgravity}{4.0cm}
 \newcommand{\axiswidthgravity}{5.0cm}
 \newcommand{\subfigurewidthgravity}{0.32\linewidth}
 \newcommand{\captionvspacegravity}{-2mm}
 
 \input{appendix.tex}
 \clearpage
 \cleardoublepage
 \bibliographystyle{plainnat}
 \bibliography{../../../Bibliography/conf_names_long,../../../Bibliography/library}
 
\end{document}
